# Supplementary material for: Characterizing videos, audience and advertising in Youtube channels for kids
Source: arXiv:1707.00971 source file (2017-07-04)
Supplement: Supplementary file 1 [file appendix.tex]

\section{Appendix}

\begin{figure}[!ht]
\centering
\includegraphics[scale=0.5]{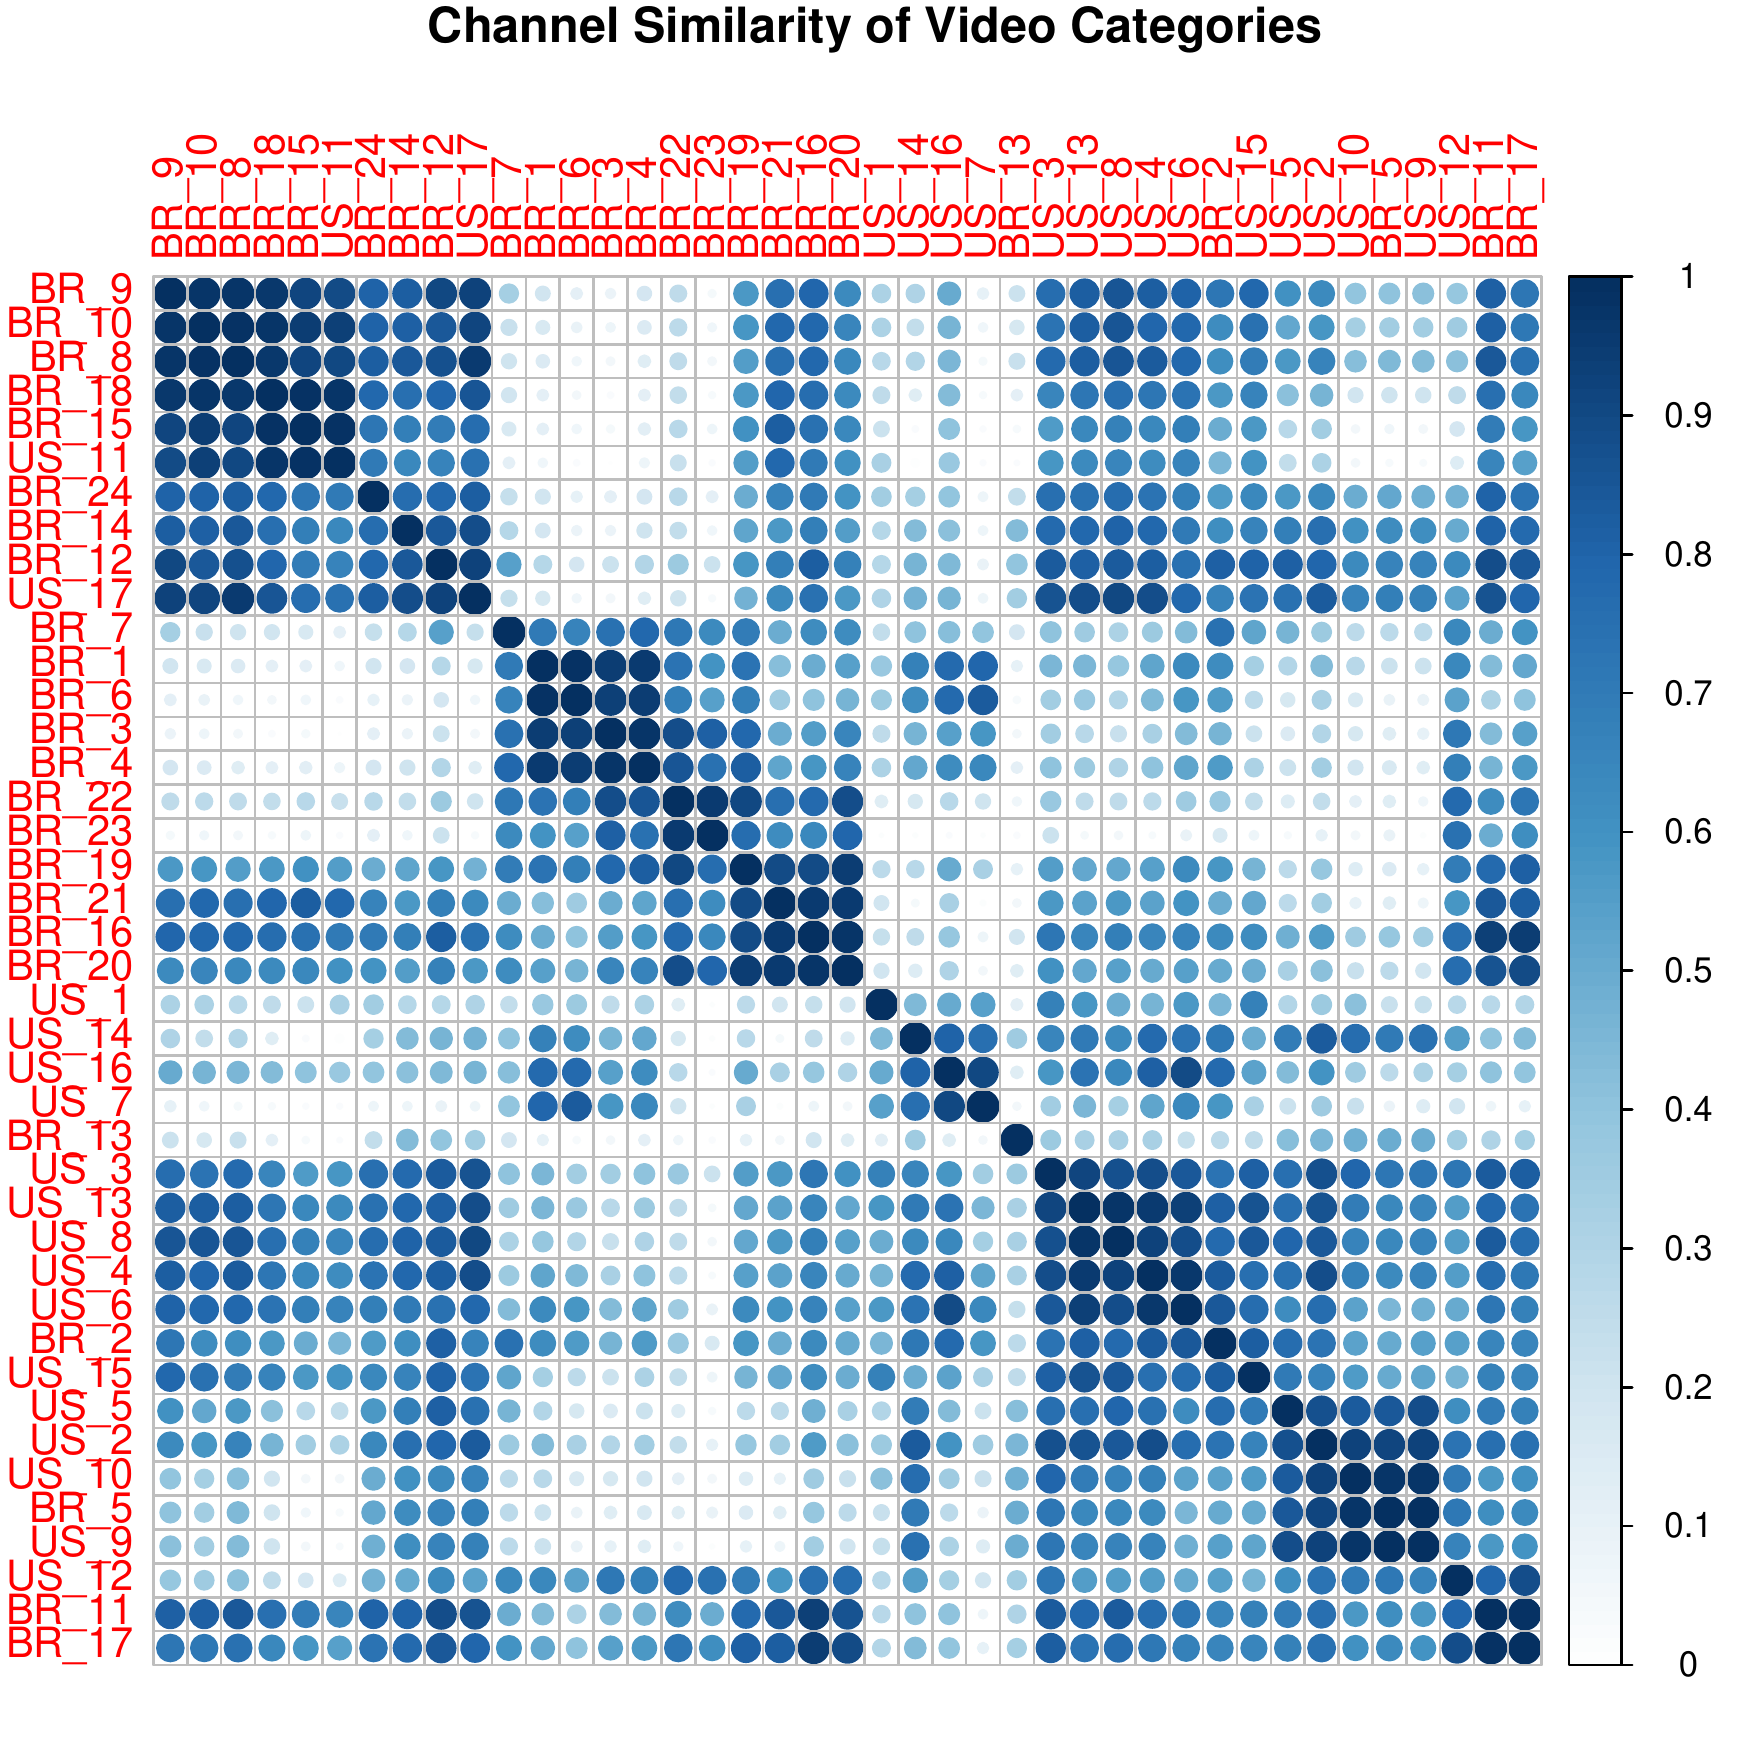}
\end{figure}

%\begin{figure}[!ht]
%\centering
%\includegraphics[scale=0.5]{fig/comments-liwc-channels.pdf}
%\end{figure}

%\begin{figure}[!ht]
%\centering
%\includegraphics[scale=0.5]{fig/comments-liwc-categories.pdf}
%\end{figure}

%\begin{figure}[!ht]
%\centering
%\includegraphics[scale=0.5]{fig/comments-liwc-gender.pdf}
%\end{figure}

%\begin{figure}[!ht]
%\centering
%\includegraphics[scale=0.5]{fig/comments-liwc-race.pdf}
%\end{figure}

%\begin{figure}[!ht]
%\centering
%\includegraphics[scale=0.5]{fig/comments-liwc-age.pdf}
%\end{figure}
